# Supplementary material for: Advanced Optimal Control Methods for Spin Systems
Source: arXiv:1803.10432 source file (2018-04-26)
Supplement: Supplementary file 1 [file awg_schematics.tikz.tex]

\begin{tikzpicture}[tight background,auto, node distance=5em,>=latex',font=\scriptsize]

\node[draw,mixer={\footnotesize{Q}}{\footnotesize\sc{lo}}{\footnotesize{I}}{\footnotesize\sc{rf}}] (IGmixer) at (0,0) {}; 
\node[draw,dir-couple=\scriptsize{dB}] (dir_couple) at (3.65,-0.235) {}; 
\node[draw,tri-buffer] (amp) at (5.6,0) {}; 
\draw ($(IGmixer.corner 270)$) to [lowpass,>,n=lp1] (3,0) to (3,0 -| dir_couple.west) node[inputarrow,rotate=0] {};
\draw (-2,0) node [oscillator](lo){} to [short] ($(IGmixer.corner 90)$) node[inputarrow,rotate=0] {};
\draw (5,0 -| dir_couple.east) to [short,>] ($(amp.corner 2)!0.5!(amp.corner 3)$) node[inputarrow,rotate=0] {};
\draw ($(amp.corner 1)$) to [short,-o] (7,0) node[right,align=center,font=\normalsize] {Shaped Pulse\\ to Resonator};
\draw (4,-1 |- dir_couple.south) to [short] (4,-1.5) to [short,-o] (6,-1.5) node[right,align=center,font=\normalsize] {Shaped Pulse to\\ Transmitter Monitor};

\node (twtlabel) at (5.675,0) {\sc{twt}};

\node (mixlabel) at (-3.75, 1.75) {\footnotesize\textcolor{gray}{\circled{2} {\sl mixer}}};
\draw (mixlabel.east) edge [-latex,out=0, in=125,dashed,shorten >=5pt,color=gray] ($(IGmixer.corner 45)$);
\node (lolabel) at (-3.75, 1.25) {\footnotesize\textcolor{gray}{\circled{1} {\sl source}}};
\draw (lolabel.east) edge [-latex,out=0, in=90,dashed,shorten >=5pt,color=gray] (lo.north);

\node (fillabel) at (8, 2) {\footnotesize\textcolor{gray}{\circled{3} {\sl filter}}};
\draw (fillabel.west) edge [-latex,out=180, in=45,dashed,shorten >=5pt,color=gray] (lp1.north);
\node (dirlabel) at (8, 1.5) {\footnotesize\textcolor{gray}{\circled{4} {\sl coupler}}};
\draw (dirlabel.west) edge [-latex,out=180, in=45,dashed,shorten >=5pt,color=gray] (dir_couple.north);
\node (twtlabels) at (8, 1) {\footnotesize\textcolor{gray}{\circled{5} {\sl travelling wave tube}}};
\draw (twtlabels.west) edge [-latex,out=180, in=90,dashed,shorten >=5pt,color=gray] ($(amp.corner 2)!0.5!(amp.corner 1)$);

\coordinate (C1) at (-1.25,-1);
\coordinate (C2) at (-1.25,2);
\path[name path=line 1] (lo) -- ($(IGmixer.corner 90)$);
\path[name path=line 2] (C2) -- (C1);
% find intersection of first and second line
  \path [name intersections={of = line 1 and line 2}];
  \coordinate (S)  at (intersection-1);

  % path a circle around this intersection for the arc
  \path[name path=circle] (S) circle(2.5pt);

  % find intersections of second line and circle
  \path [name intersections={of = circle and line 2}];
  \coordinate (I1)  at (intersection-1);
  \coordinate (I2)  at (intersection-2);

  % draw normal line segments
  \draw (I1) to[short,-o] (C2) node[above,align=center,font=\normalsize] {\sc{awg}\\Quadrature};
\draw ($(IGmixer.corner 360)$) node[inputarrow,rotate=270] {} to[short,-o] (0,1.25) node[above,align=center,font=\normalsize] {\sc{awg}\\In-Phase};
\draw ($(IGmixer.corner 180)$) node[inputarrow,rotate=90] {} to[short,-|] (0,-1) to (C1);
  \draw (I2) -- (C1);

\end{tikzpicture}
