# Supplementary material for: Advanced Optimal Control Methods for Spin Systems
Source: arXiv:1803.10432 source file (2018-04-26)
Supplement: Supplementary file 2 [file feedback_echo_convergence.tikz.tex]

\begin{tikzpicture}[tight background]%,show background rectangle]
\begin{groupplot}[conv style,
		group style={
		group size=2 by 2,
		horizontal sep=1.5em,
		vertical sep=2.25em,
		x descriptions at=edge
		  bottom,
		},
    width=\figwidth,
    xtick distance=5,
    minor x tick num = 4,
    xmin=0, xmax=15,
    groupplot xlabel={\footnotesize{{\scshape{Iteration}}}},
    ylabel={\footnotesize{{\scshape{Signal Intensity}} [{\normalfont{arb. units}}]}},
    xlabel={},
    x post scale=0.55,
    y post scale=0.7,
]
\nextgroupplot[title style={at={(0.5,1)},anchor=center,align=center},
	      title={\plotlabel{a} $^{}_{}${\scshape Quality Measure}$^{}_{}$},
	      minor y tick num = 4,
	      ymin=0, ymax=2,
	      ytick distance=0.5,
	      ylabel={Normalised \(\Obj{\objv{}}\)},
	      ylabel shift=4pt,]
	    \coordinate (top) at (rel axis cs:0,1);

            \addplot+[thick,
               solid,
               mark=none,
               color=MatlabCyan,
            ] table [x expr=\thisrow{It}, y expr=\thisrow{min}] {\datadir/AWG/xband_trityl_33pt_convergence.dat};
            \addplot+[thick,
               solid,
               mark=none,
               color=MatlabBlue,
            ] table [x expr=\thisrow{It}, y expr=\thisrow{min}] {\datadir/AWG/xband_trityl_21pt_convergence.dat};
            \addplot+[thick,
               solid,
               mark=none,
               color=MatlabGreen,
            ] table [x expr=\thisrow{It}, y expr=\thisrow{min}] {\datadir/AWG/xband_trityl_11pt_convergence.dat};
            \addplot+[thick,
               solid,
               mark=none,
               color=MatlabOrange,
            ] table [x expr=\thisrow{It}, y expr=\thisrow{min}] {\datadir/AWG/oopeseem_NMconvergence.dat};
            \addplot+[thick,
               solid,
               mark=none,
               color=MatlabRed,
            ] table [x expr=\thisrow{It}, y expr=\thisrow{min}] {\datadir/AWG/oopeseem_MDSconvergence.dat};
            \addplot[mark=none, thick, dotted, MatlabCyan, domain=11:15] {0.98299396};
            \addplot[mark=none, thick, dotted, MatlabBlue, domain=14:15] {1.26558184};
            \addplot[mark=none, thick, dotted, MatlabGreen, domain=10:15] {1.283215};
            \addplot[mark=none, thick, dotted, MatlabOrange, domain=10:15] {1.20452081};
            \addplot[mark=none, thick, dotted, MatlabRed, domain=5:15] {1.63628576};
            
\nextgroupplot[title style={at={(0.5,1)},anchor=center,align=center},
	      title={\plotlabel{b} $^{}_{}${\scshape N$^{\text{o}}$ Experiments}$^{}_{}$},
	      axis y line=right,
              tick align=outside,
              x axis line style=|-latex,
              y axis line style=-latex,
	      minor y tick num = 4,
	      ymin=0, ymax=400,
	      ytick distance=100,
	      ylabel={\#$f(\objv{})$},
	      ylabel shift=-4pt,]
	    \coordinate (top2) at (rel axis cs:0,1);

            \addplot+[thick,
               solid,
               mark=none,
               color=MatlabCyan,
            ] table [x expr=\thisrow{It}, y expr=\thisrow{no}] {\datadir/AWG/xband_trityl_33pt_convergence.dat};
            \addplot+[thick,
               solid,
               mark=none,
               color=MatlabBlue,
            ] table [x expr=\thisrow{It}, y expr=\thisrow{no}] {\datadir/AWG/xband_trityl_21pt_convergence.dat};
            \addplot+[thick,
               solid,
               mark=none,
               color=MatlabGreen,
            ] table [x expr=\thisrow{It}, y expr=\thisrow{no}] {\datadir/AWG/xband_trityl_11pt_convergence.dat};
            \addplot+[thick,
               solid,
               mark=none,
               color=MatlabOrange,
            ] table [x expr=\thisrow{It}, y expr=\thisrow{no}*2] {\datadir/AWG/oopeseem_NMconvergence.dat};
            \addplot+[thick,
               solid,
               mark=none,
               color=MatlabRed,
            ] table [x expr=\thisrow{It}, y expr=\thisrow{no}*2] {\datadir/AWG/oopeseem_MDSconvergence.dat};
            \addplot[mark=none, thick, dotted, MatlabCyan, domain=11:15] {343};
            \addplot[mark=none, thick, dotted, MatlabBlue, domain=14:15] {389};
            \addplot[mark=none, thick, dotted, MatlabGreen, domain=10:15] {119};
            \addplot[mark=none, thick, dotted, MatlabOrange, domain=10:15] {84};
            \addplot[mark=none, thick, dotted, MatlabRed, domain=5:15] {138};
            
\nextgroupplot[title style={at={(0.5,1)},anchor=center,align=center},
	      title={\plotlabel{c} $^{}_{}${\scshape Change in Quality}$^{}_{}$},
	      ymin=0.001, ymax=2,
	      ylabel={\(\Delta\Obj{\objv{}}\)},
	      ylabel shift=4pt,
	      ymode=log]

            \addplot+[thick,
               solid,
               mark=none,
               color=MatlabCyan,
            ] table [x expr=\thisrow{It}, y expr=\thisrow{change}] {\datadir/AWG/xband_trityl_33pt_convergence.dat};
            \addplot+[thick,
               solid,
               mark=none,
               color=MatlabBlue,
            ] table [x expr=\thisrow{It}, y expr=\thisrow{change}] {\datadir/AWG/xband_trityl_21pt_convergence.dat};
            \addplot+[thick,
               solid,
               mark=none,
               color=MatlabGreen,
            ] table [x expr=\thisrow{It}, y expr=\thisrow{change}] {\datadir/AWG/xband_trityl_11pt_convergence.dat};
            \addplot+[thick,
               solid,
               mark=none,
               color=MatlabOrange,
            ] table [x expr=\thisrow{It}, y expr=\thisrow{change}] {\datadir/AWG/oopeseem_NMconvergence.dat};
            \addplot+[thick,
               solid,
               mark=none,
               color=MatlabRed,
            ] table [x expr=\thisrow{It}, y expr=\thisrow{change}] {\datadir/AWG/oopeseem_MDSconvergence.dat};
            
	    \coordinate (bot2) at (rel axis cs:0,0);
	    
\nextgroupplot[title style={at={(0.5,1)},anchor=center,align=center},
	      title={\plotlabel{d} $^{}_{}${\scshape Simplex Size}$^{}_{}$},
	      axis y line=right,
              tick align=outside,
              x axis line style=|-latex,
              y axis line style=-latex,
	      ymin=0.001, ymax=2,
	      ylabel={Simplex Size},
	      ylabel shift=-4pt,
	      ymode=log,]

            \addplot+[thick,
               solid,
               mark=none,
               color=MatlabCyan,
            ] table [x expr=\thisrow{It}, y expr=\thisrow{size}] {\datadir/AWG/xband_trityl_33pt_convergence.dat};
            \addplot+[thick,
               solid,
               mark=none,
               color=MatlabBlue,
            ] table [x expr=\thisrow{It}, y expr=\thisrow{size}] {\datadir/AWG/xband_trityl_21pt_convergence.dat};
            \addplot+[thick,
               solid,
               mark=none,
               color=MatlabGreen,
            ] table [x expr=\thisrow{It}, y expr=\thisrow{size}] {\datadir/AWG/xband_trityl_11pt_convergence.dat};
            \addplot+[thick,
               solid,
               mark=none,
               color=MatlabOrange,
            ] table [x expr=\thisrow{It}, y expr=\thisrow{size}] {\datadir/AWG/oopeseem_NMconvergence.dat};
            \addplot+[thick,
               solid,
               mark=none,
               color=MatlabRed,
            ] table [x expr=\thisrow{It}, y expr=\thisrow{size}] {\datadir/AWG/oopeseem_MDSconvergence.dat};
            \addplot[mark=none, thick, dotted, MatlabCyan, domain=11:15] {343};
            \addplot[mark=none, thick, dotted, MatlabBlue, domain=14:15] {389};
            \addplot[mark=none, thick, dotted, MatlabGreen, domain=10:15] {119};
            \addplot[mark=none, thick, dotted, MatlabOrange, domain=10:15] {84};
            \addplot[mark=none, thick, dotted, MatlabRed, domain=5:15] {138};

	\coordinate (bot) at (rel axis cs:1,0);
\end{groupplot}

\path[] (top|-current bounding box.south)-- coordinate(legendpos) (bot|-current bounding box.south);
\matrix[matrix of nodes, anchor=north, inner sep=0.33em, font=\scshape\scriptsize] at (legendpos)
  {NM: 33 point echo & \draw[legendline={MatlabCyan}{1.00}] (-0.25,0.1) -- (0.25,0.1); & \hspace{2em} &
  NM: oop-eseem & \draw[legendline={MatlabOrange}{1.00}] (-0.25,0.1) -- (0.25,0.1); \\
  NM: 21 point echo & \draw[legendline={MatlabBlue}{1.00}] (-0.25,0.1) -- (0.25,0.1); & \hspace{2em} & 
  MDS: oop-eseem & \draw[legendline={MatlabRed}{1.00}] (-0.25,0.1) -- (0.25,0.1); \\
  NM: 11 point echo & \draw[legendline={MatlabGreen}{1.00}] (-0.25,0.1) -- (0.25,0.1); & \hspace{2em} & 
   & \\};

\end{tikzpicture}
